# Supplementary material for: Sampling from high-dimensional, multimodal distributions using automatically tuned, tempered Hamiltonian Monte Carlo
Source: arXiv:2111.06871 ancillary file (2025-07-29)
Supplement: Supplementary file 2 [file supp_arxiv.pdf]

# Supplementary text for *Sampling from multimodal distributions using tempered Hamiltonian transitions*

## Supplementary Content

|                                                                                                 |             |
|-------------------------------------------------------------------------------------------------|-------------|
| <b>S1 Mass-enhanced HMC with sequential proposals</b>                                           | <b>S-1</b>  |
| S1.1 Examples: mixtures of multivariate normal distributions . . . . .                          | S-2         |
| S1.2 Tuning of parameters . . . . .                                                             | S-5         |
| S1.2.1 Mass–time scale equivariance and the choice of leapfrog step size . . . . .              | S-6         |
| S1.2.2 The choice of $\alpha$ , $L$ , $N$ . . . . .                                             | S-7         |
| S1.3 Theoretical explanations of when mass-enhanced HMC does and does not work . . . . .        | S-10        |
| S1.3.1 The case where mass-enhanced HMC works . . . . .                                         | S-10        |
| S1.3.2 The case where mass-enhanced HMC does not work . . . . .                                 | S-11        |
| <b>S2 A link between tempered transitions (Neal, 1996) and tempered Hamiltonian transitions</b> | <b>S-12</b> |
| <b>S3 Additional figures for Section 4</b>                                                      | <b>S-14</b> |
| S3.1 $\eta_k = \eta_* \{1 - \cos(2\pi k/K)\}$ with $\eta_* = 0$ . . . . .                       | S-14        |
| S3.2 $\eta_k = \eta_* \{1 - \cos(2\pi k/K)\}$ with $\eta_* = 2.5$ . . . . .                     | S-16        |
| S3.3 $\eta_k = \eta_* \{1 - \cos(2\pi k/K)\}$ with $\eta_* = 3$ . . . . .                       | S-20        |

## S1 Mass-enhanced HMC with sequential proposals

In this section, we explain mass-enhanced HMC (Algorithm 0 in the main text) in detail. This method simulates the Hamiltonian dynamics for an enhanced mass  $\tilde{M} = \alpha M$  where  $\alpha > 1$ . Here  $M$  denotes the inverse covariance matrix of the multivariate normal distribution for the initial velocity. We have from (8) and (9) that the acceptance ratio for the proposed candidate  $\Psi_t(x(0), v(0); \tilde{M})$  is given by

$$e^{-H\{x(t), v(t)\} + H\{x(0), v(0)\}} \approx e^{-(1-\alpha^{-1})\{U(x(t)) - U(x(0))\}} = \left\{ \frac{\pi(x(t))}{\pi(x(0))} \right\}^{1-\alpha^{-1}},$$

which can be extremely small if  $\pi(x(t)) \ll \pi(x(0))$  and  $\alpha \gg 1$ . Thus a candidate  $(x(t), v(t))$  can be accepted for the next state of the Markov chain reasonably high probability only when  $\pi(x(t)) \gtrsim \pi(x(0))$ . A path can be simulated until such a point is found. A sequence of proposed candidates  $\{(Y_n, W_n); n \geq 1\}$  is obtained by the recursion  $(Y_n, W_n) = \Psi_t(Y_{n-1}, W_{n-1}; \tilde{M})$ , where  $(Y_0, W_0) := (x(0), v(0))$  is given by the initial position and velocity at the start of a given iteration. A candidate  $(Y_n, W_n)$  is considered acceptable if

$$\Lambda < e^{-H(Y_n, W_n) + H(Y_0, W_0)}, \tag{S1}$$

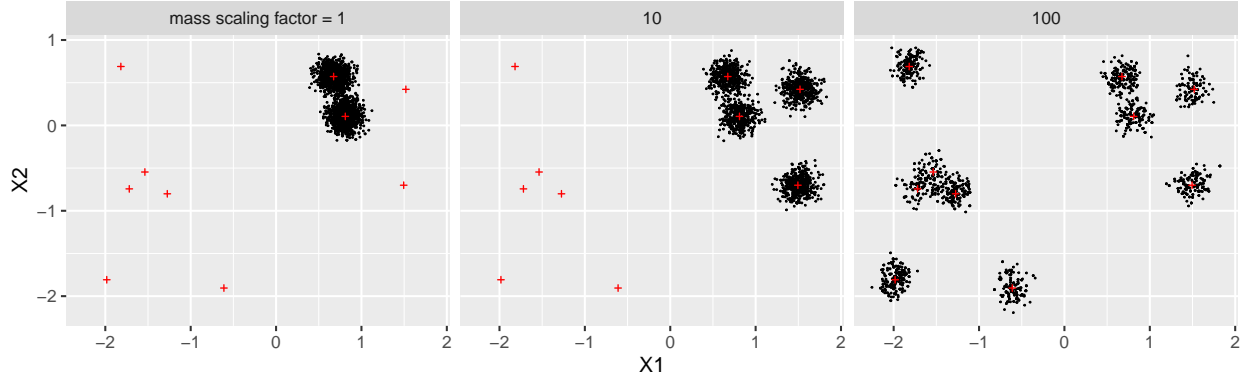

Figure S-1: Sample draws of Markov chains constructed by mass-enhanced HMC (Algorithm 0) with various mass scale factors ( $\alpha = 1, 10$ , and  $100$ ) for the target distribution considered in Example S1.1. The centers of the ten Gaussian components are marked by red '+' signs.

where a random number  $\Lambda \sim \text{Uniform}(0, 1)$  is drawn independently of all proposed candidates. The  $L$ -th acceptable proposal in the sequence  $\{(Y_n, W_n); n \geq 0\}$  is taken as the next state of the Markov chain, where  $L$  can be any number greater than or equal to one. A maximum number of  $N$  candidate proposals are made at each iteration in case the Hamiltonian path fails to reach an acceptable state. If there are less than  $L$  acceptable proposals among the first  $N$  in a given iteration, the next state of the Markov chain stays at the current state:  $X^{(i+1)} = X^{(i)}$ . This method constructs Markov chains that leave the extended target density  $\Pi(x, v)$  invariant (Park and Atchadé, 2020).

### S1.1 Examples: mixtures of multivariate normal distributions

Here we demonstrate the performance of mass-enhanced HMC (Algorithm 0) for mixtures of normal distributions. Examples S1.1 and S1.2 show that the method can construct globally mixing Markov chains for mixtures of high-dimensional normal distributions in the special case where all mixture components have the same covariance that is equal to the mass matrix  $M$ . Example S1.3 show that in general, however, the method may fail if the mixture covariances are different.

We first note that if every mixture component has the same covariance given by  $\Sigma$ , then by choosing the mass matrix  $M$  equal to  $\Sigma^{-1}$ , one can effectively turn the target distribution into a mixture of normal components with a shared covariance  $I$ . To see this, consider a transformation of variables

$$x' := \Sigma^{-1/2}x, \quad v' := \Sigma^{-1/2}v \quad (\text{S2})$$

where  $\Sigma^{-1/2}$  is the inverse of the symmetric square-root matrix of  $\Sigma$ . This linear transformation make the target distribution a mixture of normal components with covariance  $I$ . These transformed variables  $(x', v')$  satisfy the Hamiltonian equation of motion with unit mass, as follows:

$$\begin{aligned} \frac{dx'}{dt} &= \Sigma^{-1/2} \frac{dx}{dt} = v', \\ \frac{dv'}{dt} &= \Sigma^{-1/2} \frac{dv}{dt} = -\Sigma^{-1/2} \cdot M^{-1} \frac{\partial U}{\partial x} = -\Sigma^{1/2} \frac{\partial U}{\partial x} = -\frac{\partial U}{\partial x'}. \end{aligned}$$

Thus for the case where all mixture components have the same covariance, we can without loss of generality assume that the common covariance is equal to  $I$ .

**Example S1.1** Figure S-1 shows the sample draws for a two-dimensional mixture distribution of ten Gaussian components. The target density is given by

$$\pi(x) = \frac{1}{10} \sum_{j=1}^{10} \phi(x; \mu_j, \sigma^2 I), \quad x \in \mathbb{R}^2,$$

where the centers of the density components  $\mu_j$ ,  $j \in 1:10$ , are distributed randomly across the square  $[-2, 2]^2$  as shown in Figure S-1. The standard deviation of each component  $\sigma$  was 0.1. We constructed Markov chains of length two thousand using Algorithm 0 with three different values of the mass scale factors,  $\alpha = 1, 10$ , and 100. The leapfrog step size varied linearly with the square root of the mass scale factor ( $\tilde{\epsilon} = 0.1 \cdot \sqrt{\alpha}$ ). The first acceptable proposal was taken for the next state of the Markov chain (i.e.,  $L = 1$ ), and each iteration was terminated if no acceptable proposal was found among the first  $N = 10$  proposals. The inverse covariance matrix for the velocity distribution was equal to the identity matrix ( $M = I$ ). The numerical results shown in Figure S-1 show that using mass enhancement ratio  $\alpha > 1$  can enable jumps between separated density components. When we run sequential-proposal HMC *without* mass enhancing (i.e.,  $\alpha = 1$ ), the Markov chain could reach only one density component nearest to the initial component. When  $\alpha = 10$ , the sample Markov chain reached more density components but not remotely separated ones. When  $\alpha = 100$ , the chain reached all components.  $\square$

**Example S1.2** Next we demonstrate how Algorithm 0 scales with increasing space dimension  $d$ . Since it is sufficient to demonstrate that the algorithm facilitates jumps from one density component to another, we set the target distribution to be a mixture of two Gaussian components where the distance between the center of the components and the standard deviation of both components are fixed:

$$\pi_d(x_d) = \frac{1}{2} \sum_{j=1}^2 \phi(x_d; \mu_{j,d}, \sigma^2 I_d), \quad x_d \in \mathbb{R}^d, \quad (\text{S3})$$

where  $\|\mu_{1,d} - \mu_{2,d}\| = 2$ ,  $\sigma \equiv 0.1$  for  $d = 2, 20$ , and 200. The directions of  $\mu_{1,d} - \mu_{2,d}$  were randomly generated from spherically uniform distributions. We ran both a standard HMC and mass-enhanced HMC (Algorithm 0) for these target distributions. For mass-enhanced HMC, the mass enhancement ratio was  $\alpha = 100$ , the number of acceptable proposals found in each iteration was  $L = 1$ , and the maximum number of proposals in each iteration was  $N = 1000$ . The mass-enhanced HMC method was run for  $I = 2000$  iterations, and the standard HMC method was run for roughly the same amount of time. Each proposal in mass-enhanced HMC was obtained by extending the numerical simulation by one leapfrog step. The proposals in HMC were obtained by making five leapfrog jump steps with a randomly drawn initial velocity. The leapfrog step size of 0.1 was used.

Figure S-2b shows the closest density component (1 or 2) for each state of the Markov chains constructed by both methods. Whereas the Markov chains constructed by standard HMC failed to jump from one density component to the other, the Markov chains constructed by mass-enhanced HMC made frequent jumps between the density components. Figure S-2a shows the states in the constructed Markov chains, projected to the direction connecting the two density modes (i.e.,  $\mu_{2,d} - \mu_{1,d}$ ) and to a randomly selected direction perpendicular to  $\mu_{2,d} - \mu_{1,d}$ . Standard HMC drew samples from only one density component, but mass-enhanced HMC was able to sample from both density components. Considering that the second density component has most of its mass on an exponentially small part of the  $d$  dimensional target space, we think mass-enhanced HMC shows a remarkable efficiency in finding in a remote density component in high dimensions. As pointed out previously, this is due to the fact that the mass-enhanced HMC method searches the target space by exploiting the geometry of the log target density function via the Hamiltonian dynamics.  $\square$

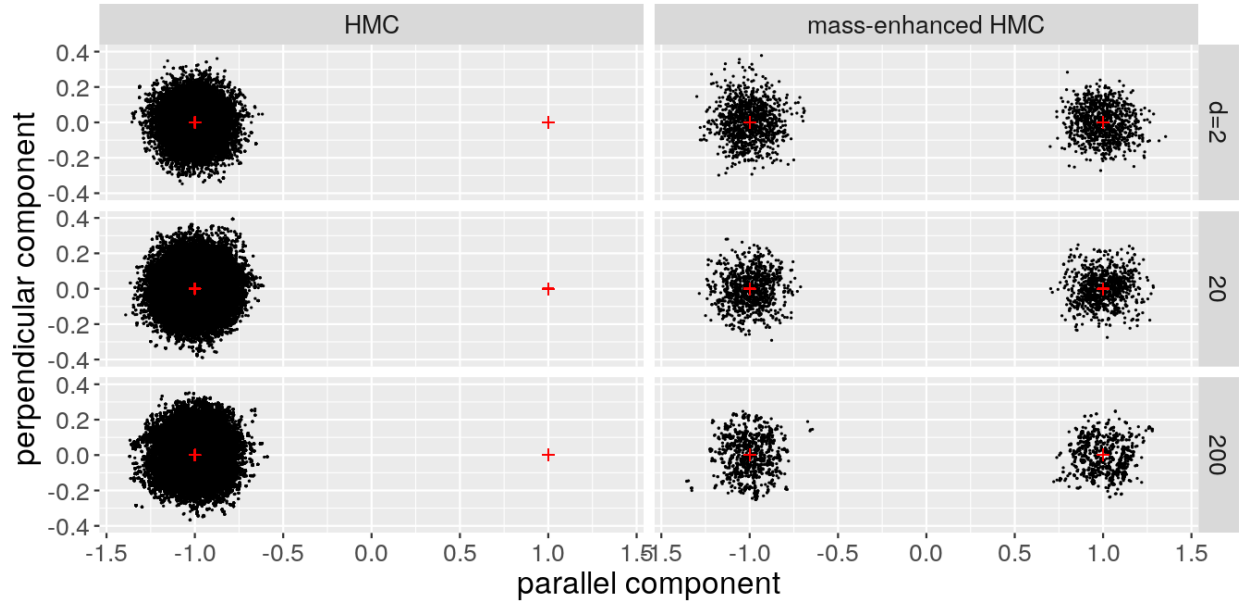

(a) Sample draws of the constructed Markov chains. The  $x$ -axis shows the projection onto the direction from one density mode to the other (i.e.,  $\mu_{2,d} - \mu_{1,d}$ ), and the  $y$ -axis shows the projection onto a randomly selected direction perpendicular to  $\mu_{2,d} - \mu_{1,d}$ . The experimental settings are the same as those in Figure S-2b.

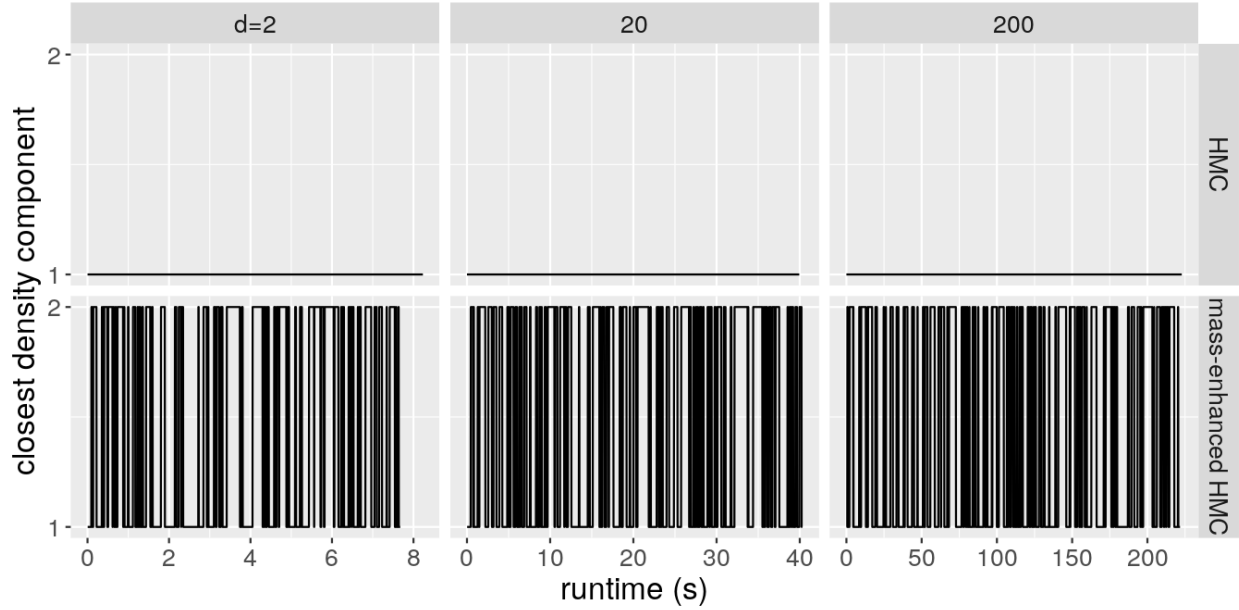

(b) The closest density component (1 or 2) for each state of the constructed Markov chains. The number of algorithm iterations ( $I$ ) was two thousand for mass-enhanced HMC, and HMC was run for approximately the same amount of time. The leapfrog step size of 0.1 was used for both HMC and mass-enhanced HMC. For mass-enhanced HMC, the number of acceptable candidates searched for in each iteration was  $L = 1$ ; maximum number of proposed candidates per iteration was  $N = 1000$ ; mass enhancement ratio was  $\alpha = 100$ .

Figure S-2: Markov chains constructed by HMC and mass-enhanced HMC (Algorithm 0) where the target density is given by (S3) ( $d = 2, 20, 200$ ).

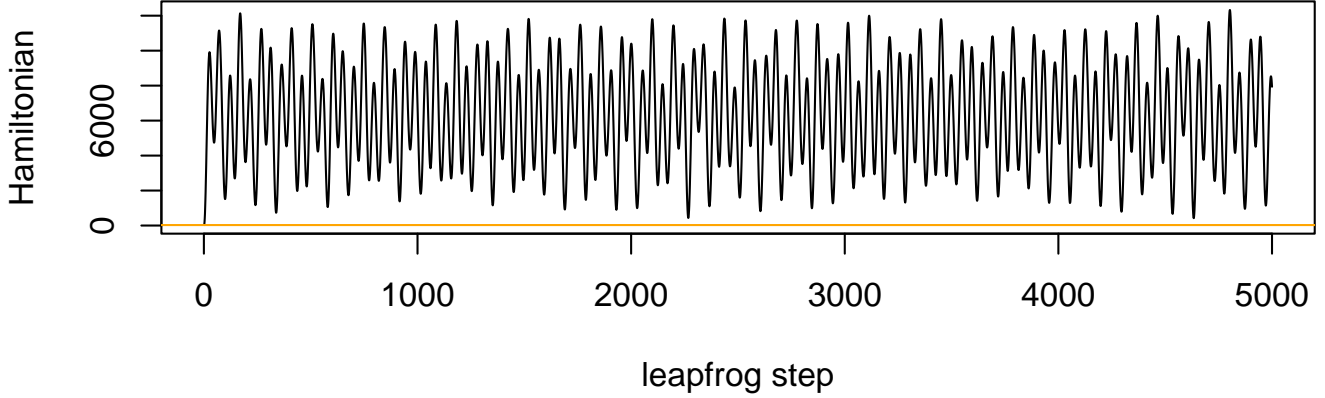

Figure S-3: The Hamiltonian evaluated along an example path for the ten-dimensional Gaussian target distribution  $\mathcal{N}(0, \Sigma)$  considered in Example S1.3 where the mass matrix  $M$  is not equal to  $\Sigma$ .

The tuning of the leapfrog step size, as well as other parameters in Algorithm 0 such as  $\alpha$ ,  $L$ , and  $N$ , will be discussed in Section S1.2.

**Example S1.3** Previous examples showed that when the mixture components have the same covariance, mass-enhanced HMC can construct Markov chains that hop frequently between the components. Example S1.2 in particular showed that the method works well for high-dimensional target distributions. In general, however, when the mixture components have different covariances, mass-enhanced HMC fails to facilitate jumps between the components. This motivated the main algorithm of this paper (Algorithm 1, tempered Hamiltonian transitions).

If the covariances of the mixture components are not the same, then obviously, the mass matrix  $M$  cannot be equal to the inverse of every mixture covariance. Therefore it suffices to show that if  $M$  is not equal to the inverse of the covariance matrix  $\Sigma$ , mass-enhanced HMC fails. For simplicity, we consider a Gaussian target distribution, that is, a mixture consisting of a single component. Without loss of generality, we let the covariance  $\Sigma$  be a diagonal matrix. The target space dimension is ten, and the square roots of the diagonal entries of  $\Sigma$  are randomly drawn from the uniform distribution between 0.5 and 4. The mass matrix  $M$  is equal to the identity matrix, and the mass-scaling factor  $\alpha$  is equal to 2000. Starting from a point randomly drawn from the target distribution  $\mathcal{N}(0, \Sigma)$ , an example path was simulated with mass  $\tilde{M} = \alpha M = 2000I$  and leapfrog step size  $\tilde{\epsilon} = 0.1\sqrt{\alpha} = \sqrt{20}$ . The Hamiltonian evaluated at every leapfrog step is shown in Figure S-3. The Hamiltonian values are consistently higher than the initial value indicated by the yellow horizontal line. This result indicates that when the mass matrix  $M$  is not equal to the inverse of the covariance matrix, the simulated paths with enhanced mass may not reach an acceptable state for a very long time. A theoretical analysis shows that this is the case in general when  $M$  is not a scalar multiple of  $\Sigma^{-1}$  (see Section S1.3.2).  $\square$

## S1.2 Tuning of parameters

### S1.2.1 Mass–time scale equivariance and the choice of leapfrog step size

We consider a transformation of variables that offers insight into tuning of the leapfrog step size for mass-enhanced HMC. The following lemma is a consequence of what we call *mass–time scale equivariance* (see Section 2.3 in the main text).

**Lemma S1.** *The leapfrog method constructs the same path when simulating the Hamiltonian dynamics with  $M$ , initial velocity  $v(0)$ , and step size  $\epsilon$  and when simulating it with mass  $\tilde{M} = \alpha M$ , initial velocity  $\alpha^{-1/2}v(0)$ , and step size  $\tilde{\epsilon} = \alpha^{1/2}\epsilon$ .*

*Proof.* Consider a transformation of variables given by

$$\begin{aligned}\tilde{t} &= \alpha^{1/2}t, \\ \tilde{x}(\tilde{t}) &= x(t), \\ \tilde{v}(\tilde{t}) &= \alpha^{-1/2}v(t).\end{aligned}\tag{S4}$$

Then we can see that the following differential equations hold:

$$\begin{aligned}\frac{d\tilde{x}}{d\tilde{t}} &= \alpha^{-1/2}\frac{dx}{dt} = \alpha^{-1/2}v = \tilde{v}, \\ \frac{d\tilde{v}}{d\tilde{t}} &= \frac{\alpha^{-1/2}}{\alpha^{1/2}}\frac{dv}{dt} = \alpha^{-1}M^{-1}\frac{\partial U}{\partial x} = \tilde{M}^{-1}\frac{\partial U}{\partial \tilde{x}}.\end{aligned}\tag{S5}$$

Thus the transformed variables  $(\tilde{x}(\tilde{t}), \tilde{v}(\tilde{t}))$  is a solution to the same differential equations as the HEM (7) with mass  $\tilde{M}$ . This mass–time scale equivariance implies that the discrete-time numerical simulation described by (4) with LF step size

$$\tilde{\epsilon} = \alpha^{1/2}\epsilon$$

and initial state  $(\tilde{x}(0), \tilde{v}(0)) = (x(0), \alpha^{-1/2}v(0))$  and mass  $\tilde{M}$  constructs the same path as the LF numerical simulation with mass  $M$ , initial condition  $(x(0), v(0))$ , and step size  $\epsilon$ . We can see this explicitly from the following equations:

$$\begin{aligned}\tilde{v}\left(\tilde{t} + \frac{\tilde{\epsilon}}{2}\right) &= \alpha^{-1/2}v\left(t + \frac{\epsilon}{2}\right) = \alpha^{-1/2}v(t) - \alpha^{-1/2}\frac{\epsilon}{2}M^{-1}\nabla U(x(t)) \\ &= \tilde{v}(\tilde{t}) - \frac{\tilde{\epsilon}}{2}(\alpha M)^{-1}\nabla U(\tilde{x}(\tilde{t})), \\ \tilde{x}(\tilde{t} + \tilde{\epsilon}) &= x(t + \epsilon) = x(t) + \epsilon v\left(t + \frac{\epsilon}{2}\right) \\ &= x(t) + \alpha^{-1/2}\tilde{\epsilon}\alpha^{1/2}\tilde{v}\left(\tilde{t} + \frac{\tilde{\epsilon}}{2}\right) \\ &= \tilde{x}(\tilde{t}) + \tilde{\epsilon}\tilde{v}\left(\tilde{t} + \frac{\tilde{\epsilon}}{2}\right), \\ \tilde{v}(\tilde{t} + \tilde{\epsilon}) &= \alpha^{-1/2}v(t + \epsilon) = \alpha^{-1/2}v\left(t + \frac{\epsilon}{2}\right) - \alpha^{-1/2}\frac{\epsilon}{2}M^{-1}\nabla U(x(t + \epsilon)) \\ &= \tilde{v}\left(\tilde{t} + \frac{\tilde{\epsilon}}{2}\right) - \frac{\tilde{\epsilon}}{2}(\alpha M)^{-1}\nabla U(\tilde{x}(\tilde{t} + \tilde{\epsilon})).\end{aligned}$$

Furthermore, since there is a one-to-one correspondence between the coordinate systems  $(t, x, v)$  and  $(\tilde{t}, \tilde{x}, \tilde{v})$ , the numerical simulation of  $(\tilde{t}, \tilde{x}, \tilde{v})$  is stable if and only if the numerical simulation of  $(t, x, v)$  is stable.  $\square$

| Parameter  | Description                                                  | Tuning guidelines                                                                                                                                                                               |
|------------|--------------------------------------------------------------|-------------------------------------------------------------------------------------------------------------------------------------------------------------------------------------------------|
| $\alpha$   | Mass scale factor                                            | The simulated paths should be able to reach the desired search scope for isolated modes.                                                                                                        |
| $\epsilon$ | Leapfrog step size                                           | As large as possible while ensuring that the numerical simulation is stable ( $\tilde{\epsilon} = \sqrt{\alpha} \cdot \epsilon$ ).                                                              |
| $L$        | Number of acceptable proposals to be found in each iteration | Large enough so that the simulated path can escape the local basin it starts from.                                                                                                              |
| $N$        | Maximum number of proposals to be made in each iteration     | Large enough so that the simulated path can reach a new density component, while ensuring that the algorithm is not excessively slowed down in case $v(0)$ and $\Lambda$ are drawn unfavorably. |

Table S-1: Tuning guidelines for parameters in Algorithm 0

Lemma S1 suggests a tuning of the leapfrog step size given by  $\tilde{\epsilon} = \sqrt{\alpha}\epsilon$  for Algorithm 0. However, we note that Algorithm 0 simulates the HEM with the initial velocity  $v(0)$  instead of  $\tilde{v}(0) = \alpha^{-1/2}v(0)$ . Thus it constructs the same as that obtained by numerically simulating the Hamiltonian dynamics with mass  $M$  and *increased* initial velocity  $\alpha^{1/2}v(0)$ . The mass-time scale equivariance (S4) shows that the following two ways of enhancing the initial kinetic energy  $K(v(0)) = \frac{1}{2}v(0)^\top M v(0)$  by a factor of  $\alpha$  are equivalent:

1. increase the mass from  $M$  to  $\alpha M$ , or
2. increase the initial velocity from  $v(0)$  to  $\alpha^{1/2}v(0)$ .

If the curvature of the potential energy function is not constant, the suggested scaling  $\tilde{\epsilon} = \sqrt{\alpha}\epsilon$  may lead to numerical instability, because the Hessian at  $x(\epsilon) = x(0) + \epsilon\alpha^{1/2}v(0)$  may differ greatly from the Hessian at  $x(0)$ . In this case,  $\tilde{\epsilon}$  may need to be chosen smaller than  $\alpha^{1/2}\epsilon$ .

### S1.2.2 The choice of $\alpha$ , $L$ , $N$

In mass-enhanced HMC with sequential proposals (Algorithm 0), the mass scale factor  $\alpha$  implicitly determines the search scope for separated density components. Since  $U(x(t)) + \tilde{K}(v(t))$  is approximately conserved on the simulated path, every point on the path satisfies

$$U(x(t)) \lesssim U(x(0)) + \alpha K(v(0)), \quad (\text{S6})$$

where  $K(v(0)) \sim \frac{1}{2}\chi_d^2$ . Therefore, with increasing  $\alpha$ , the area reachable by the simulated paths are expanded, and the depth of the potential energy barrier that can be crossed is increased.

**Example S1.4** Figure S-4 shows the simulated Hamiltonian paths with mass enhancement ratios  $\alpha = 1, 30$ , and 200 where the target distribution  $\pi$  is a mixture of two Gaussian density components:

$$\pi(x) = \frac{1}{2}\phi\{x; (-4, -1), I_{2 \times 2}\} + \frac{1}{2}\phi\{x; (4, 1), I_{2 \times 2}\}. \quad (\text{S7})$$

Here  $\phi(x; \mu, I_{2 \times 2})$  denotes the multivariate Gaussian density with mean  $\mu$  and the covariance matrix equal to the two dimensional identity matrix. All three paths start with the same initial velocity  $v(0)$ . The points on the numerically simulated paths are marked by orange dots if they are acceptable according to the criteria  $H(x, v) < H\{x(0), v(0)\} - \log \Lambda$ , where the Uniform(0,1) random number  $\Lambda$  is assumed to take value 0.5. Figure S-5 plots the potential energy, the kinetic energy, and the Hamiltonian



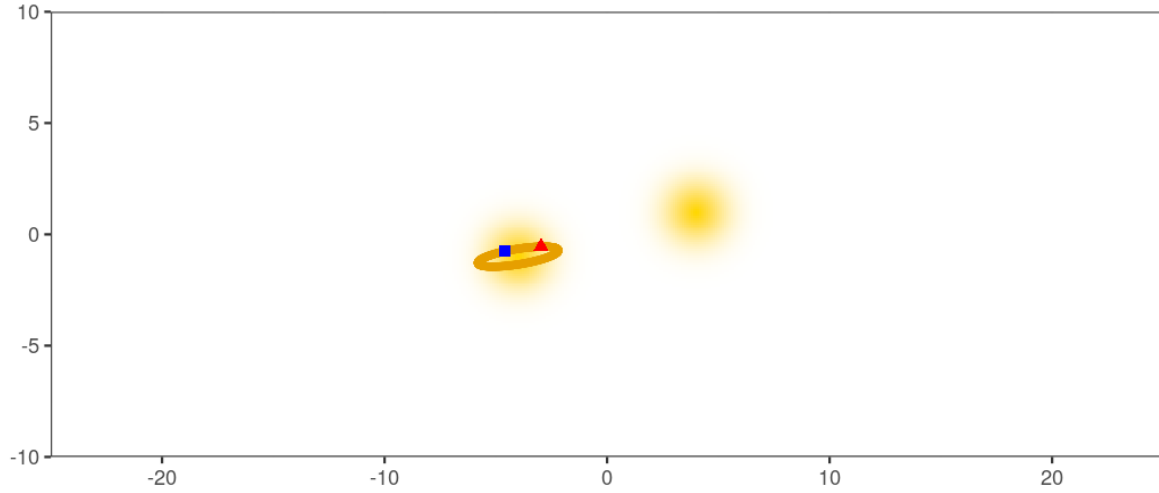

(a)  $\alpha = 1$

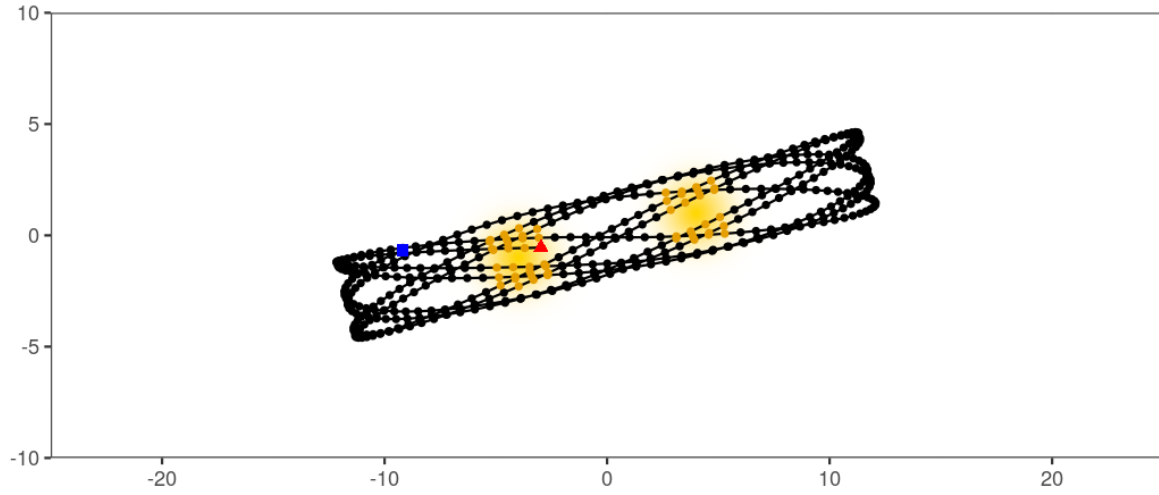

(b)  $\alpha = 30$

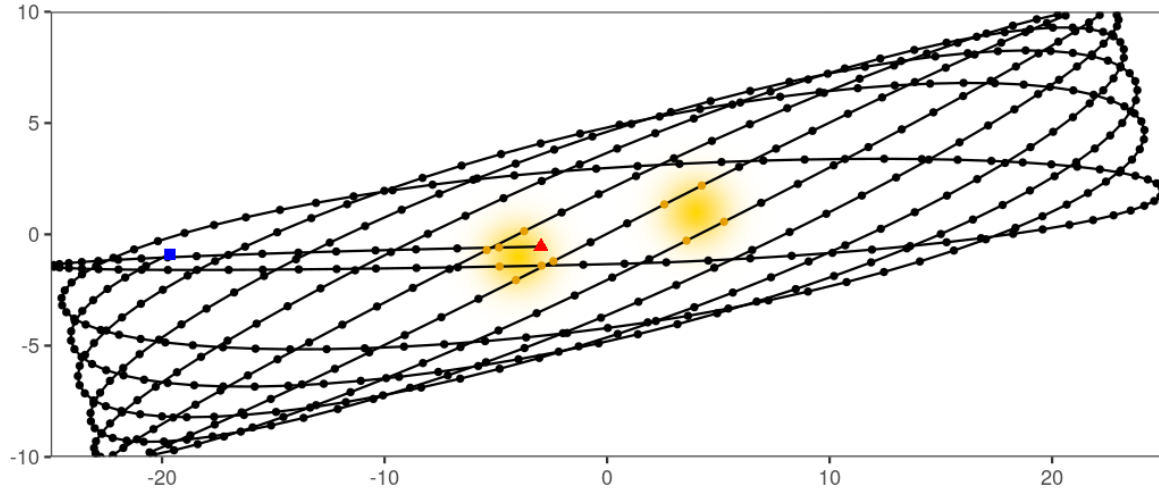

(c)  $\alpha = 200$

Figure S-4: Numerically simulated Hamiltonian paths with varied mass scale factor  $\alpha$  for a mixture of two normal target density considered in Example S1.4. The two modes of the target distribution are represented by yellow color gradient. Acceptable points when the uniform  $(0, 1)$  random number  $\Lambda$  is equal to 0.5 is shown as orange dots. The initial position is marked by a red triangle, and the 500-th position by a blue square.



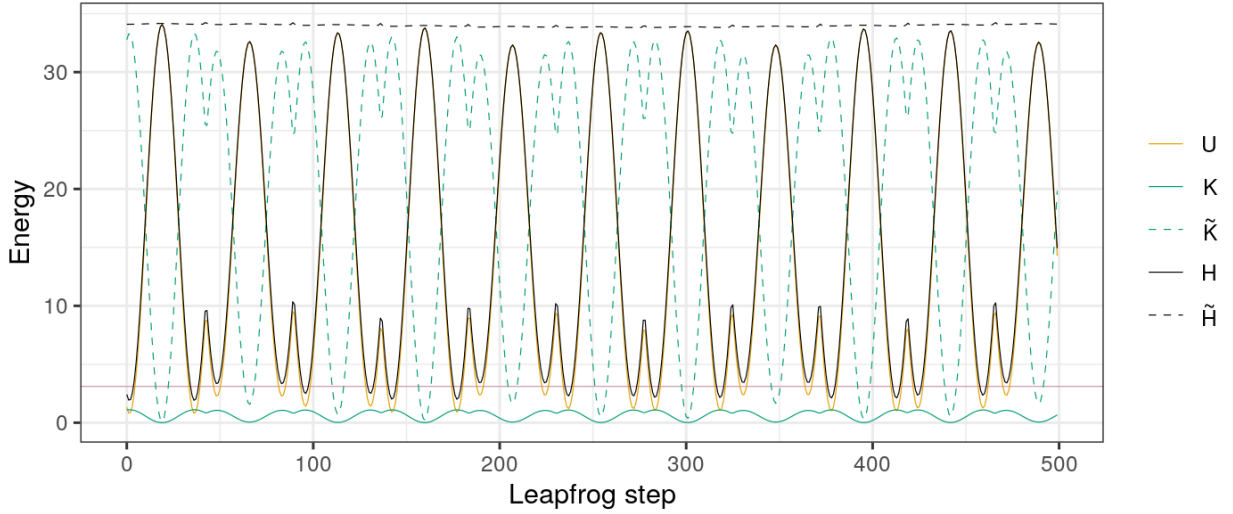

Figure S-5: The traceplots for  $U(x(t))$ ,  $K(v(t))$ ,  $\tilde{K}(v(t))$ ,  $H\{x(t), v(t)\}$ , and  $\tilde{H}\{x(t), v(t)\}$  for the simulated path shown in Figure S-4b. The horizontal line at around 3 marks the acceptability criterion  $H\{x(0), v(0)\} - \log(0.5)$ , assuming that  $\Lambda = 0.5$ .

of the points along the simulated path where the mass is either  $M$  or  $\tilde{M} = \alpha M$  where  $\alpha = 30$ . The Hamiltonian  $H$  with mass  $\tilde{M}$ , indicated by the dashed black line, is approximately constant, but the Hamiltonian  $\tilde{H}$  with mass  $M$ , indicated by the solid black line, fluctuates depending on the proportions of  $\tilde{H}$  made up by the potential energy  $U$  and the kinetic energy  $\tilde{K}$ . A point on the path is acceptable if the Hamiltonian  $H$  is less than  $H(x(0), v(0)) - \log \Lambda$ , which is indicated by the green horizontal line.

When  $\alpha = 1$  (Figure S-4a), the Hamiltonian path does not leave the density component where the current state of the Markov chain is located. However, the simulated paths can move across the region of low target density between the two modes when  $\alpha = 30$  (Figure S-4b). If  $\alpha$  is even greater ( $\alpha = 200$ ), the simulated Hamiltonian path reaches a wider area (Figure S-4c). Since the simulated path traverses a wider area when  $\alpha = 200$ , the proportion of acceptable states along the path may be smaller than when  $\alpha = 30$ . Thus tuning  $\alpha = 30$  may lead to more efficient sampling than  $\alpha = 200$  for this target density given by (S7). However, if there was another density component at a remote location (say at  $(-20, -5)$ ), the simulation with  $\alpha = 200$  would be able to reach it whereas that with  $\alpha = 30$  would not. Therefore, the mass enhancement ratio  $\alpha$  may be chosen based on the desired search scope for isolated modes. The search area is dependent on the geometry of the surface of the log target density function. In Figure S-4b and S-4c, the simulated Hamiltonian paths stay along the direction connecting the two density modes, where the potential energy is relatively low. Algorithm 0 is assisted by the local geometry of the potential energy landscape so that it can efficiently search for isolated modes regardless of the space dimension.

Insight into the simulated paths can be gained by looking at the traceplot of  $H\{x(t), v(t)\}$ . Figure S-5 shows the traceplots for  $U(x(t))$ ,  $K(v(t))$ ,  $H\{x(t), v(t)\}$ ,  $\tilde{K}(v(t))$ , and  $\tilde{H}\{x(t), v(t)\}$  for the simulated path for  $\alpha = 30$  (Figure S-4b). The value of  $\tilde{H}\{x(t), v(t)\} = U(x(t)) + \tilde{K}(v(t))$  is approximately constant, whereas the value of  $H\{x(t), v(t)\}$  is mostly affected by  $U(x(t))$ . For numerically stable paths,  $U(x(t))$  and  $K(v(t))$  should have oscillatory traceplots. Acceptable points are those for which  $H\{x(t), v(t)\}$  is less than  $H\{x(0), v(0)\} - \log \Lambda$ , and those points occur periodically.  $\square$

The parameter  $L$  in Algorithm 0 should be chosen large enough that the simulated path may leave the local mode it starts from. This makes it more likely that the next state of the constructed Markov chain, which is the  $L$ -th acceptable proposal along the path, is found in a different density component. In Figure S-4b, the simulated path starts from the red triangle and leaves the acceptable region around

the first density component in four steps. Thus in this case, if  $L$  is suitably large, say  $L \geq 4$ , the next state of the constructed Markov chain may be found near the other mode located at  $(4, 1)$ .

The parameter  $N$  sets an upper bound on the simulation time per iteration. Therefore, it needs to be large enough to allow the simulated path to reach a remote density component. However, in some cases such as when the log density surface is flat, the simulated path may head to a wrong direction for a prolonged amount of time. Moreover, in rare cases where the current state of the Markov chain is close to the maximum of the target density and the drawn uniform random number  $\Lambda$  is close to one, acceptable points may only be found in a very small area of  $\mathbf{X}$  where the target density is higher than the starting point. The parameter  $N$  needs to be set appropriately so as to avoid spending an excessive amount of time on finding an acceptable candidate in these unfavorable cases. Table S-1 summarizes the parameters in the algorithm and guidelines for tuning parameters.

### S1.3 Theoretical explanations of when mass-enhanced HMC does and does not work

#### S1.3.1 The case where mass-enhanced HMC works

The fact that mass-enhanced HMC can construct globally mixing Markov chains for high-dimensional target distributions of the form

$$\pi(x) = \frac{1}{2} \sum_{j=1}^2 \phi(x; \mu_j, I), \quad x \in \mathbb{R}^d$$

as in Example S1.2 can be mathematically explained as follows. The target density is proportional to

$$\pi(x) \propto e^{-\|x-\mu_1\|^2/2} + e^{-\|x-\mu_2\|^2/2} =: c_1(x) + c_2(x),$$

where without loss of generality we assume that

$$\mu_1 = (\mu_1^1, 0, \dots, 0), \quad \mu_2 = (\mu_2^1, 0, \dots, 0).$$

For simplicity we suppose  $M = I$ . We have

$$\frac{\partial U}{\partial x} = -\frac{\partial}{\partial x} \log \pi(x) = \frac{c_1(x) \cdot (x - \mu_1) + c_2(x) \cdot (x - \mu_2)}{c_1(x) + c_2(x)},$$

or

$$\frac{\partial U}{\partial x_i} = \begin{cases} \frac{c_1(x)(x_1 - \mu_1^1) + c_2(x)(x_1 - \mu_2^1)}{c_1(x) + c_2(x)} & \text{for } i = 1 \\ x_i & \text{for } i \geq 2. \end{cases}$$

Thus for  $i \geq 2$  the Hamiltonian equations of motion for  $(x_i, v_i)$  can be solved independently:

$$\frac{dx_i}{dt} = v_i, \quad \frac{dv_i}{dt} = -\tilde{M}^{-1} \frac{\partial U}{\partial x_i} = -\alpha^{-1} x_i.$$

The solution is given by

$$x_i(t) = A_i \sin(\omega t + \varphi_i), \quad v_i(t) = A_i \omega \cos(\omega t + \varphi_i)$$

where  $\omega = \sqrt{\alpha^{-1}}$ . The amplitude  $A_i$  satisfies

$$A_i^2 = x_i(0)^2 + \omega^{-2} v_i(0)^2 = x_i(0)^2 + \alpha v_i(0)^2,$$

and the initial phase  $\varphi_i \in [0, 2\pi)$  satisfies

$$x_i(0) = A_i \sin(\varphi_i), \quad v_i(0) = A_i \omega \cos(\varphi_i)$$

Since  $\omega = \sqrt{\alpha^{-1}} \gg 1$  and both  $x_i(0)$  and  $v_i(0)$  are random draws from  $\mathcal{N}(0, 1)$ , the value of  $\sin \varphi$  is close to zero and  $\cos \varphi$  is close to one.

For  $i = 1$ , we can consider a division of the space into three regions,  $R_1 = \{x; c_1(x) \gg c_2(x)\}$ ,  $R_2 = \{x; c_1(x) \ll c_2(x)\}$ , and  $R_3 = (R_1 \cup R_2)^c$ . Since both  $c_1(x)$  and  $c_2(x)$  are exponential quadratic functions of  $x$ , most points in the space belongs to either the first or the second region. Suppose without loss of generality that  $x(0)$  belongs to  $R_1$ . In this region,  $(x_1(t), v_1(t))$  approximately has a similar form as that for  $i \leq 2$ , namely

$$x_1(t) - \mu_1^1 = A_1 \sin(\omega t + \varphi_1), \quad v_1(t) = A_1 \omega \cos(\omega t + \varphi_1).$$

As the path enters the region  $R_3$ , the amplitude and the phase change in a way that is hard to predict, but after the path passes through  $R_3$  and enters  $R_2$  the solution becomes again approximately sinusoidal:

$$x_1(t) - \mu_2^1 = A'_1 \sin(\omega t + \varphi'_1), \quad v_1(t) = A'_1 \omega \cos(\omega t + \varphi'_1).$$

The Hamiltonian in  $R_2$  can be expressed as

$$\begin{aligned} H(t) &\approx \frac{1}{2} \|x - \mu_2\|^2 + \frac{1}{2} \|v\|^2 \\ &= \frac{1}{2} (x_1 - \mu_2^1)^2 + \frac{1}{2} v_1(t)^2 + \sum_{i \geq 2} \left[ \frac{1}{2} x_i(t)^2 + \frac{1}{2} v_i(t)^2 \right] \\ &= \left\{ \frac{1}{2} A_1'^2 \sin^2(\omega t + \varphi'_1) + \frac{1}{2} A_1'^2 \omega^2 \cos^2(\omega t + \varphi'_1) \right\} + \left\{ \sum_{i \geq 2} \left[ \frac{1}{2} A_i^2 \sin^2(\omega t + \varphi_i) + \frac{1}{2} A_i^2 \omega^2 \cos^2(\omega t + \varphi_i) \right] \right\} \\ &:= H_1(t) + H_{i \geq 2}(t) \end{aligned}$$

Since the angular frequency is the same and equal to  $\omega$  for all  $i \geq 2$ , the second term can be expressed as

$$H_{i \geq 2}(t) = B^0 + B^1 \cos(2\omega t + \theta) \tag{S8}$$

for some constants  $B^0, B^1$ , and  $\theta$ . Therefore,  $\Delta H_{i \geq 2}(t) := H_{i \geq 2}(t) - H_{i \geq 2}(0)$  periodically becomes zero or negative value with frequency  $\omega/\pi$ , regardless of the dimension  $d$ . The quantity  $H_1(t)$  is also periodic with frequency  $\omega/\pi$ . Therefore if  $\varphi'_1$  is such that both  $\Delta H_1(t)$  and  $\Delta H_{i \geq 2}(t)$  can be simultaneously small at some point, that point can be accepted with a reasonably large probability. As  $\alpha$  increases,  $H_{i \geq 2}(0)$  becomes closer to the minimum of its cycle, and the combined phase  $\theta$  in (S8) approaches  $\pi$ . Thus the range of  $\omega t$  for which  $\Delta H_{i \geq 2}$  is below zero becomes narrower, and the chance that a point is accepted during the time a path stays in  $R_2$  decreases. In this case, many re-entering into  $R_2$  may be necessary before the phase  $\varphi'_1$  takes a fortunate value that allows a point on the path to be accepted. In conclusion, as the distance between the two modes  $\|\mu_1 - \mu_2\|$  increases, a larger value of  $\alpha$  will need to be used in order to enable the simulated path to reach a different mode, and the probability of accepted jump from one mode to another decreases. However, the jump probability is not sensitive to the space dimension  $d$ ; this conclusion is consistent with the results shown in Figure S-2.

### S1.3.2 The case where mass-enhanced HMC does not work

Now we consider the case where mass-enhanced HMC does not work well; Example S1.3 illustrates this case. Consider again a unimodal Gaussian distribution  $\mathcal{N}(0, \Sigma)$  where  $\Sigma$  is not equal to a scalar multiple

of the mass inverse matrix  $M^{-1}$ . Using the linear transformation (S2), we can simplify the case such that  $M = I$  and  $\Sigma$  is anisotropic (i.e., not a scalar multiple of the identity matrix). Without loss of generality, suppose that  $\Sigma$  is diagonal with entries  $\sigma_{ii}^2$ ,  $i = 1, \dots, d$  and that these  $d$  variances are all different. The solution to the Hamiltonian equations of motion

$$\frac{dx_i}{dt} = v_i, \quad \frac{dv_i}{dt} = -\tilde{M}^{-1} \frac{\partial U}{\partial x_i} = -\alpha^{-1} \sigma_{ii}^{-2} x_i$$

for the  $i$ -th component is given by

$$x_i(t) = A_i \sin(\omega_i t + \varphi_i), \quad v_i(t) = A_i \omega_i \cos(\omega_i t + \varphi_i)$$

where  $\omega_i = \sqrt{\alpha^{-1} \sigma_{ii}^{-1}}$ . If  $\alpha \gg 1$ , the  $d$  components are almost in sync, because

$$\frac{\sin(\varphi_i)}{\cos(\varphi_i)} = \frac{x_i(0)}{v_i(0)} \omega_i = \frac{x_i(0)}{v_i(0)} \sqrt{\alpha^{-1} \sigma_{ii}^{-1}} \approx 0, \quad \forall i.$$

However, as time progresses, the  $d$  components become asynchronized due to the fact that  $\omega_i$  are all different. It takes an exponentially long time in  $d$  for all the components to be in sync again. Therefore for  $\alpha \gg 1$  and large  $d$ , the increase in Hamiltonian  $\Delta H(t)$  is consistently large for a very long time. This phenomenon was demonstrated by Example S1.3.

## S2 A link between tempered transitions (Neal, 1996) and tempered Hamiltonian transitions

(Neal, 1996) developed an MCMC method that applies to a given state a sequence of transition kernels that have distributions at varying levels of temperature as their stationary distributions. There is an increased chance that the end state is in a different mode than the mode the initial state was in, due to this series of tempered transitions. The sequence of states are denoted by

$$\hat{x}_0 \xrightarrow{T_1} \hat{x}_1 \xrightarrow{T_2} \cdots \hat{x}_{n-1} \xrightarrow{T_n} \bar{x}_n \xrightarrow{\tilde{T}_n} \check{x}_{n-1} \xrightarrow{\tilde{T}_{n-1}} \cdots \check{x}_1 \xrightarrow{\tilde{T}_1} \check{x}_0,$$

where  $\hat{x}_0$  is the initial state and  $\check{x}_0$  is the final state, which becomes the proposed candidate for the next state of the Markov chain constructed by the method. The transition kernels  $T_1, \dots, T_n, \tilde{T}_n, \dots, \tilde{T}_1$  satisfy the relationship

$$p_k(x_k) dx_k T_k(x_k, dx'_k) = p_k(x'_k) dx'_k \tilde{T}_k(x'_k, dx_k) \quad (\text{S9})$$

where  $p_k(x_k)$  denotes the density of the  $i$ -th auxiliary distribution. The density of the target distribution that we want to sample from is denoted by  $p_0(x)$ . The auxiliary distributions often represent the distribution at various temperature levels; for example, we may have  $p_k(x) \propto p_0^{\beta_k}(x)$  where  $\beta_k$  denotes the  $i$ -th inverse temperature. This choice is made to facilitate global mixing, but the method has the target  $p_0$  as its stationary distribution for any choice of  $\{p_k; 1 \leq k \leq N\}$ . The acceptance probability for the proposed candidate  $\check{x}_0$  is given by

$$\min \left[ 1, \frac{p_1(\hat{x}_0)}{p_0(\hat{x}_0)} \cdot \frac{p_2(\hat{x}_1)}{p_1(\hat{x}_1)} \cdots \frac{p_n(\hat{x}_{n-1})}{p_{n-1}(\hat{x}_{n-1})} \cdot \frac{p_{n-1}(\check{x}_{n-1})}{p_n(\check{x}_{n-1})} \cdots \frac{p_0(\check{x}_0)}{p_1(\check{x}_0)} \right]. \quad (\text{S10})$$

In practice, the kernels  $T_k$  and  $\tilde{T}_k$  are often constructed using the Metropolis-Hastings strategy. For example, a sequence of proposal kernels  $Q_k$  can be used to draw

$$\hat{x}_0 \xrightarrow{Q_1} \hat{x}_1 \xrightarrow{Q_2} \cdots \hat{x}_{n-1} \xrightarrow{Q_n} \bar{x}_n \xrightarrow{Q_{n+1}} \check{x}_{n-1} \xrightarrow{Q_{n+2}} \cdots \check{x}_1 \xrightarrow{Q_{2n}} \check{x}_0. \quad (\text{S11})$$

Accepting each state in the sequence using the Metropolis-Hastings ratios of the form

$$\frac{p_k(\hat{x}_k)d\hat{x}_kQ_k(\hat{x}_k,d\hat{x}_{k-1})}{p_k(\hat{x}_{k-1})d\hat{x}_{k-1}Q_{2n-k+1}(\hat{x}_{k-1},\hat{x}_k)} \quad \text{or} \quad \frac{p_k(\check{x}_{k-1})d\check{x}_{k-1}Q_k(\check{x}_{k-1},d\check{x}_k)}{p_k(\check{x}_k)d\check{x}_kQ_{2n-k+1}(\check{x}_k,d\check{x}_{k-1})} \quad (\text{S12})$$

lead to the construction of the transition kernels  $T_k$  and  $\tilde{T}_k$  satisfying (S9). Here we understand  $\hat{x}_n = \check{x}_n = \bar{x}_n$ . Instead of accepting or rejecting each state on the sequence, we can continue drawing  $\hat{x}_1, \dots, \bar{x}_n, \dots, \check{x}_0$  using the proposal kernels  $Q_1, \dots, Q_{2n}$  and combine the ratios of the form (S12) with the acceptance ratio in (S10). The combined acceptance probability for the final state  $\check{x}_0$  is given by

$$\min \left[ 1, \frac{p_0(\check{x}_0)d\check{x}_0Q_1(\check{x}_0,d\check{x}_1) \cdots Q_n(\check{x}_{n-1},d\bar{x}_n)Q_{n+1}(\bar{x}_n,d\hat{x}_{n-1}) \cdots Q_{2n}(\hat{x}_1,d\hat{x}_0)}{p_0(\hat{x}_0)d\hat{x}_0Q_1(\hat{x}_0,d\hat{x}_1) \cdots Q_n(\hat{x}_{n-1},d\bar{x}_n)Q_{n+1}(\bar{x}_n,d\check{x}_{n-1}) \cdots Q_{2n}(\check{x}_1,d\check{x}_0)} \right].$$

Tempered Hamiltonian transitions (Algorithm 1) can be thought of as a special case of tempered transitions (S11) where the states  $\hat{x}_k$  or  $\check{x}_k$  are given by the pair  $(x_k, \tilde{v}_k)$  for  $k \in 0 : 2n$  and where the kernel  $Q_k(x_{k-1}, \tilde{v}_{k-1}; dx_k d\tilde{v}_k)$  puts all its mass at point

$$\Psi_{\tilde{\epsilon}_{k-\frac{1}{2}}}(x_{k-1}, \tilde{v}_{k-1}; \alpha_{k-\frac{1}{2}}M, \tilde{\epsilon}_{k-\frac{1}{2}}),$$

which is obtained by the deterministic simulation of the Hamiltonian dynamics for mass  $\alpha_{k-\frac{1}{2}}M$  by one step of the leapfrog method with step size  $\tilde{\epsilon}_{k-\frac{1}{2}} = \alpha_{k-\frac{1}{2}}^{\frac{2}{\gamma+2}}$  where the choice of  $\gamma$  was discussed in Section 3.3. The case where the proposal kernels  $Q_1, \dots, Q_{2n}$  are symmetric in the sense that  $Q_j = Q_{2n+1-j}$  for  $j \in 1 : n$  corresponds to the case where the initial value of  $k(=k_0)$  in Algorithm 1 is equal to zero. The initial and final densities are given by

$$p_0(x_0, \tilde{v}_0) = e^{-U(x_0)} \det \left( \frac{\alpha_0 M}{2\pi} \right)^{1/2} e^{-\tilde{v}_0^\top (\alpha_0 M) \tilde{v}_0 / 2},$$

$$p_{2n}(x_{2n}, \tilde{v}_{2n}) = e^{-U(x_{2n})} \det \left( \frac{\alpha_{2n} M}{2\pi} \right)^{1/2} e^{-\tilde{v}_{2n}^\top (\alpha_{2n} M) \tilde{v}_{2n} / 2}.$$

In order to explain the acceptance probability for the final pair, we view the sequence of transitions in the following way:

$$\begin{aligned} (x_1, \tilde{v}_1) &= \Psi_{\tilde{\epsilon}_{\frac{1}{2}}}(x_0, \tilde{v}_0; \alpha_{\frac{1}{2}}M, \tilde{\epsilon}_{\frac{1}{2}}) \\ (x_2, \tilde{v}_2) &= \Psi_{\tilde{\epsilon}_{\frac{3}{2}}}(x_1, \tilde{v}_1; \alpha_{\frac{3}{2}}M, \tilde{\epsilon}_{\frac{3}{2}}) \\ &\dots \\ (x_n, \tilde{v}_n) &= \Psi_{\tilde{\epsilon}_{n-\frac{1}{2}}}(x_{n-1}, \tilde{v}_{n-1}; \alpha_{n-\frac{1}{2}}M, \tilde{\epsilon}_{n-\frac{1}{2}}) \\ (x_n, \tilde{v}'_n) &= \mathcal{T}(x_n, \tilde{v}_n) = (x_n, -\tilde{v}_n) \\ (x_{n+1}, \tilde{v}'_{n+1}) &= \Psi_{-\tilde{\epsilon}_{n+\frac{1}{2}}}(x_n, \tilde{v}'_n; \alpha_{n+\frac{1}{2}}M, \tilde{\epsilon}_{n+\frac{1}{2}}) \\ &\dots \\ (x_{2n}, \tilde{v}'_{2n}) &= \Psi_{-\tilde{\epsilon}_{2n-\frac{1}{2}}}(x_{2n-1}, \tilde{v}_{2n-1}; \alpha_{2n-\frac{1}{2}}M, \tilde{\epsilon}_{2n-\frac{1}{2}}) \end{aligned}$$

Here  $\mathcal{T}$  is the velocity reflection operator. Since

$$(x_{n+1}, \tilde{v}'_{n+1}) = \Psi_{-\tilde{\epsilon}_{n+\frac{1}{2}}}(x_n, \tilde{v}'_n; \alpha_{n+\frac{1}{2}}M, \tilde{\epsilon}_{n+\frac{1}{2}}) = \mathcal{T} \circ \Psi_{\tilde{\epsilon}_{n+\frac{1}{2}}}(x_n, \tilde{v}_n; \alpha_{n+\frac{1}{2}}M, \tilde{\epsilon}_{n+\frac{1}{2}}) = (x_{n+1}, -\tilde{v}_{n+1})$$

and the same relation holds recursively for all subsequent transitions, we see that  $\tilde{v}'_{n+m} = -\tilde{v}_{n+m}$  for  $m \in 0 : n$ . The reason that we view the sequence of transitions this way is the following symmetry:

$$\begin{aligned}(x_{2n}, \tilde{v}'_{2n}) &= \Psi_{-\tilde{\epsilon}_{2n-\frac{1}{2}}} \circ \cdots \circ \Psi_{-\tilde{\epsilon}_{n+\frac{1}{2}}} \circ \mathcal{T} \circ \Psi_{\tilde{\epsilon}_{n-\frac{1}{2}}} \circ \cdots \circ \Psi_{\tilde{\epsilon}_1}(x_0, \tilde{v}_0) \\ (x_0, \tilde{v}_0) &= \Psi_{-\tilde{\epsilon}_{\frac{1}{2}}} \circ \cdots \circ \Psi_{-\tilde{\epsilon}_{n-\frac{1}{2}}} \circ \mathcal{T} \circ \Psi_{\tilde{\epsilon}_{n+\frac{1}{2}}} \circ \cdots \circ \Psi_{\tilde{\epsilon}_{2n-\frac{1}{2}}}(x_{2n}, \tilde{v}'_{2n})\end{aligned}$$

The acceptance probability for  $(x_{2n}, \tilde{v}'_{2n})$  is given by

$$\frac{p_{2n}(x_{2n}, \tilde{v}'_{2n}) dx_{2n} d\tilde{v}'_{2n} \delta_{\Psi_{\tilde{\epsilon}_{2n-\frac{1}{2}}}(x_{2n}, \tilde{v}'_{2n})}(dx_{2n-1} d\tilde{v}'_{2n-1}) \cdots \delta_{\Psi_{-\tilde{\epsilon}_{\frac{1}{2}}}(x_1, \tilde{v}_1)}(dx_0 d\tilde{v}_0)}{p_0(x_0, \tilde{v}_0) dx_0 d\tilde{v}_0 \delta_{\Psi_{\tilde{\epsilon}_{\frac{1}{2}}}(x_0, \tilde{v}_0)}(dx_1 d\tilde{v}_1) \cdots \delta_{\Psi_{-\tilde{\epsilon}_{2n-\frac{1}{2}}}(x_{2n-1}, \tilde{v}'_{2n-1})}(dx_{2n} d\tilde{v}'_{2n})} = \frac{p_{2n}(x_{2n}, \tilde{v}'_{2n})}{p_0(x_0, \tilde{v}_0)} \left| \frac{d(x_{2n}, \tilde{v}'_{2n})}{d(x_0, \tilde{v}_0)} \right| \dots \quad (\text{S13})$$

Since the leapfrog method preserves the volume element  $dx d\tilde{v}$  and  $\tilde{v}'_n = -\tilde{v}_n$ , the Jacobian determinant in the right hand side of (S13).

## S3 Additional figures for Section 4

In this supplementary section, we give some additional figures for Section 4.

### S3.1 $\eta_k = \eta_* \{1 - \cos(2\pi k/K)\}$ with $\eta_* = 0$

Figure S-6 shows that when there is no mass scaling in Algorithm 1 (i.e., the mass scale factor is constant and equal to unity), the constructed Markov chains only explore one of the local modes of the posterior distribution of the sensor locations ( $R^2$  and  $\sigma_e^2$  are assumed to be known as in Section 4.1). Some of the local modes reached by the independent chains are not one of the two dominant modes, indicating that the poor global mixing leads not only to the absence of mode hops, but to incorrect representation of the posterior distribution.



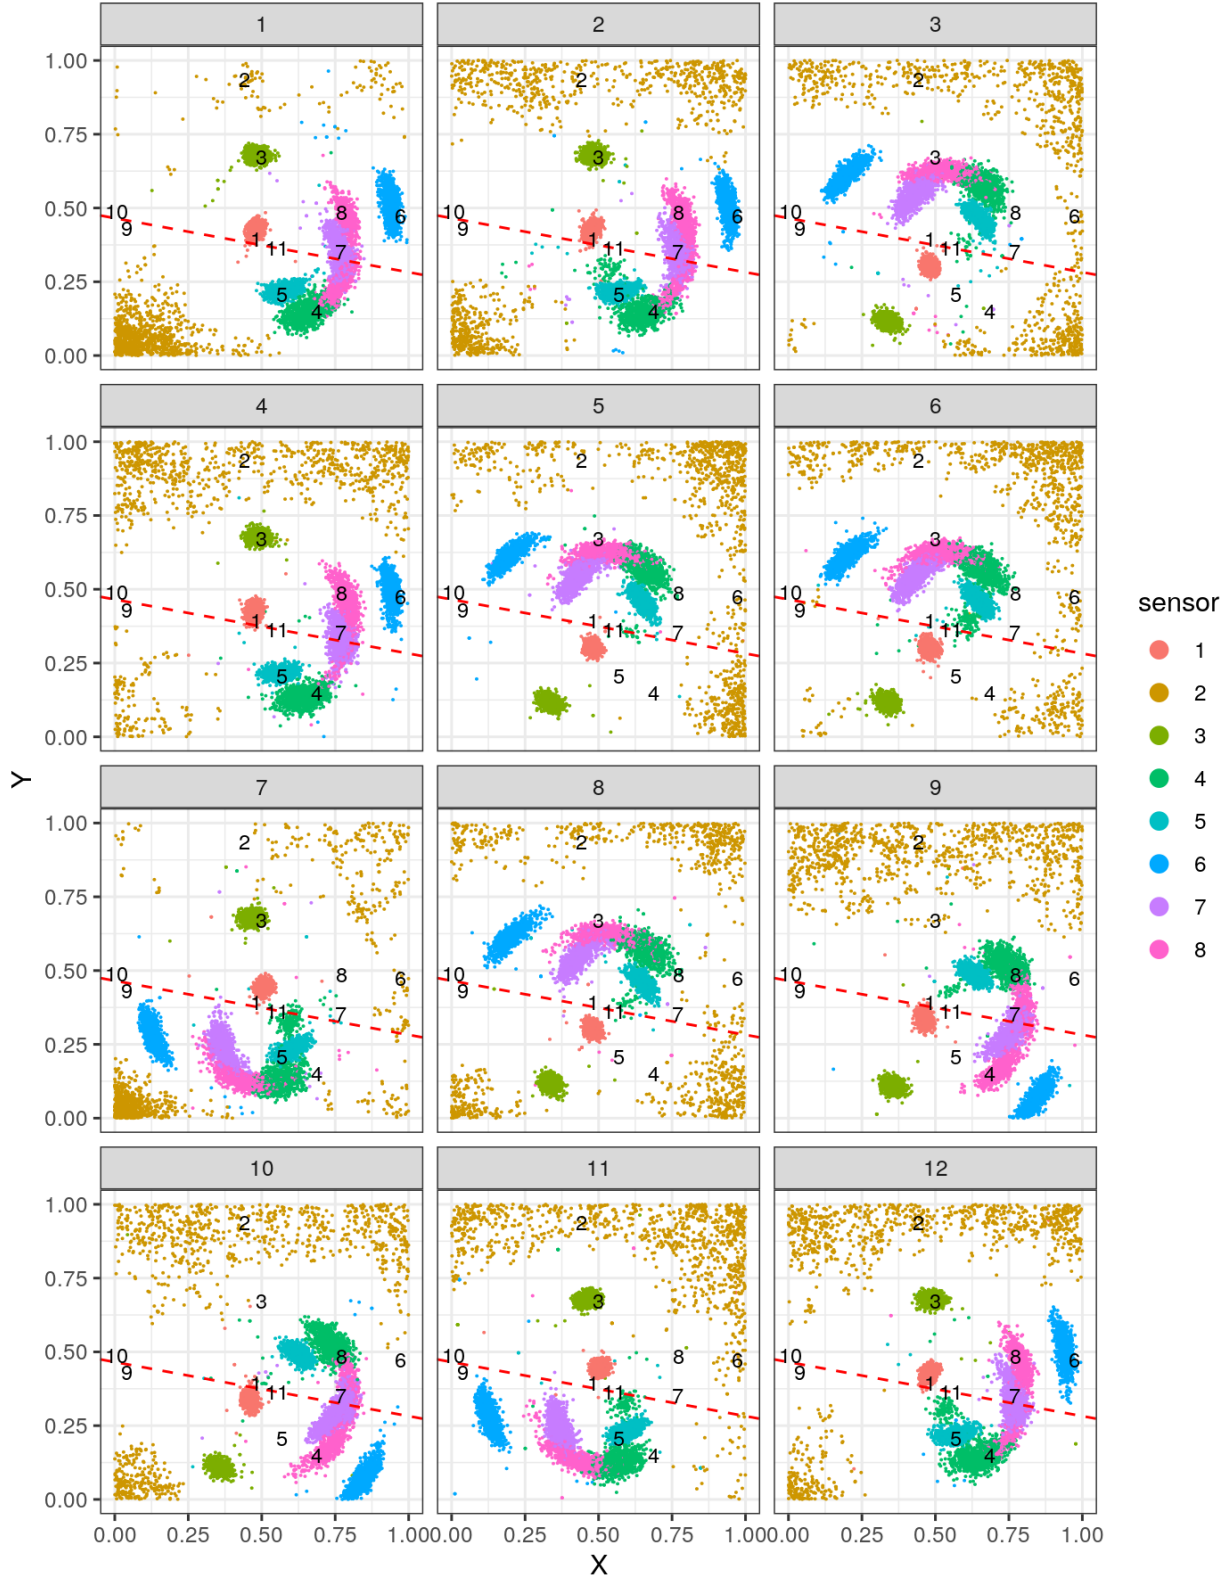

Figure S-6: The marginal posterior draws for the sensor locations from twelve independent Markov chains constructed without using mass scaling. These Markov chains were constructed using Algorithm 1 where  $\eta_k = \eta_* \{1 - \cos(2\pi k/K)\}$  with  $\eta_* = 0$  and  $K = 2000$ . The true location of each sensor is marked on the plot by its number. Sensors 9, 10, and 11 had known locations.



### S3.2 $\eta_k = \eta_* \{1 - \cos(2\pi k/K)\}$ with $\eta_* = 2.5$

Figures S-7–S-9 show that the Markov chains constructed by Algorithm 1 when the maximum mass scale factor is equal to  $e^{4\eta_*} = e^{10}$  are able to jump between the two dominant modes of the posterior distribution. The results for  $\eta_* = 2.5$  and  $\eta_* = 3$  (Section S3.3) show that Algorithm 1 is reasonably robust with respect to the tuning of the maximum mass scale factor, provided that it is large enough to enable hops between modes.

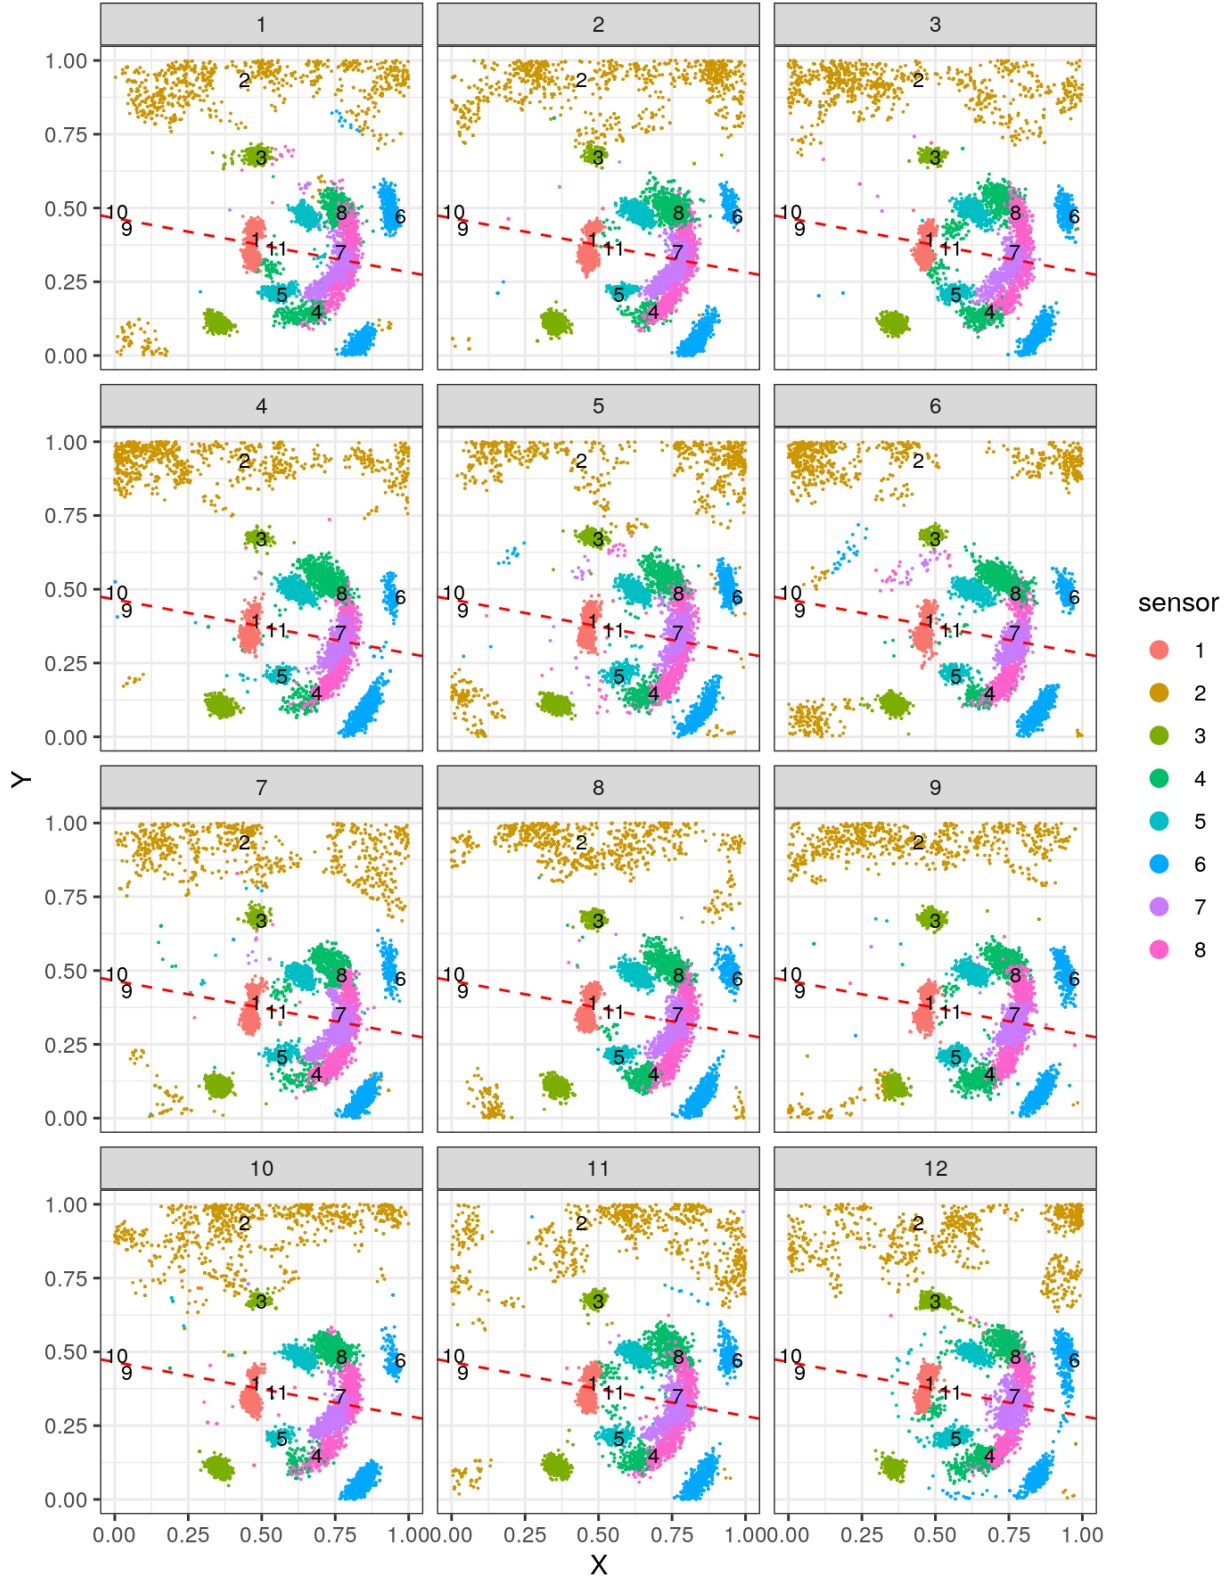

Figure S-7: The marginal posterior draws for the sensor locations from twelve independent Markov chains constructed using Algorithm 1 where  $\eta_k = \eta_* \{1 - \cos(2\pi k/K)\}$  with  $\eta_* = 2.5$  and  $K = 2000$ . The true location of each sensor is marked on the plot by its number. Sensors 9, 10, and 11 had known locations.

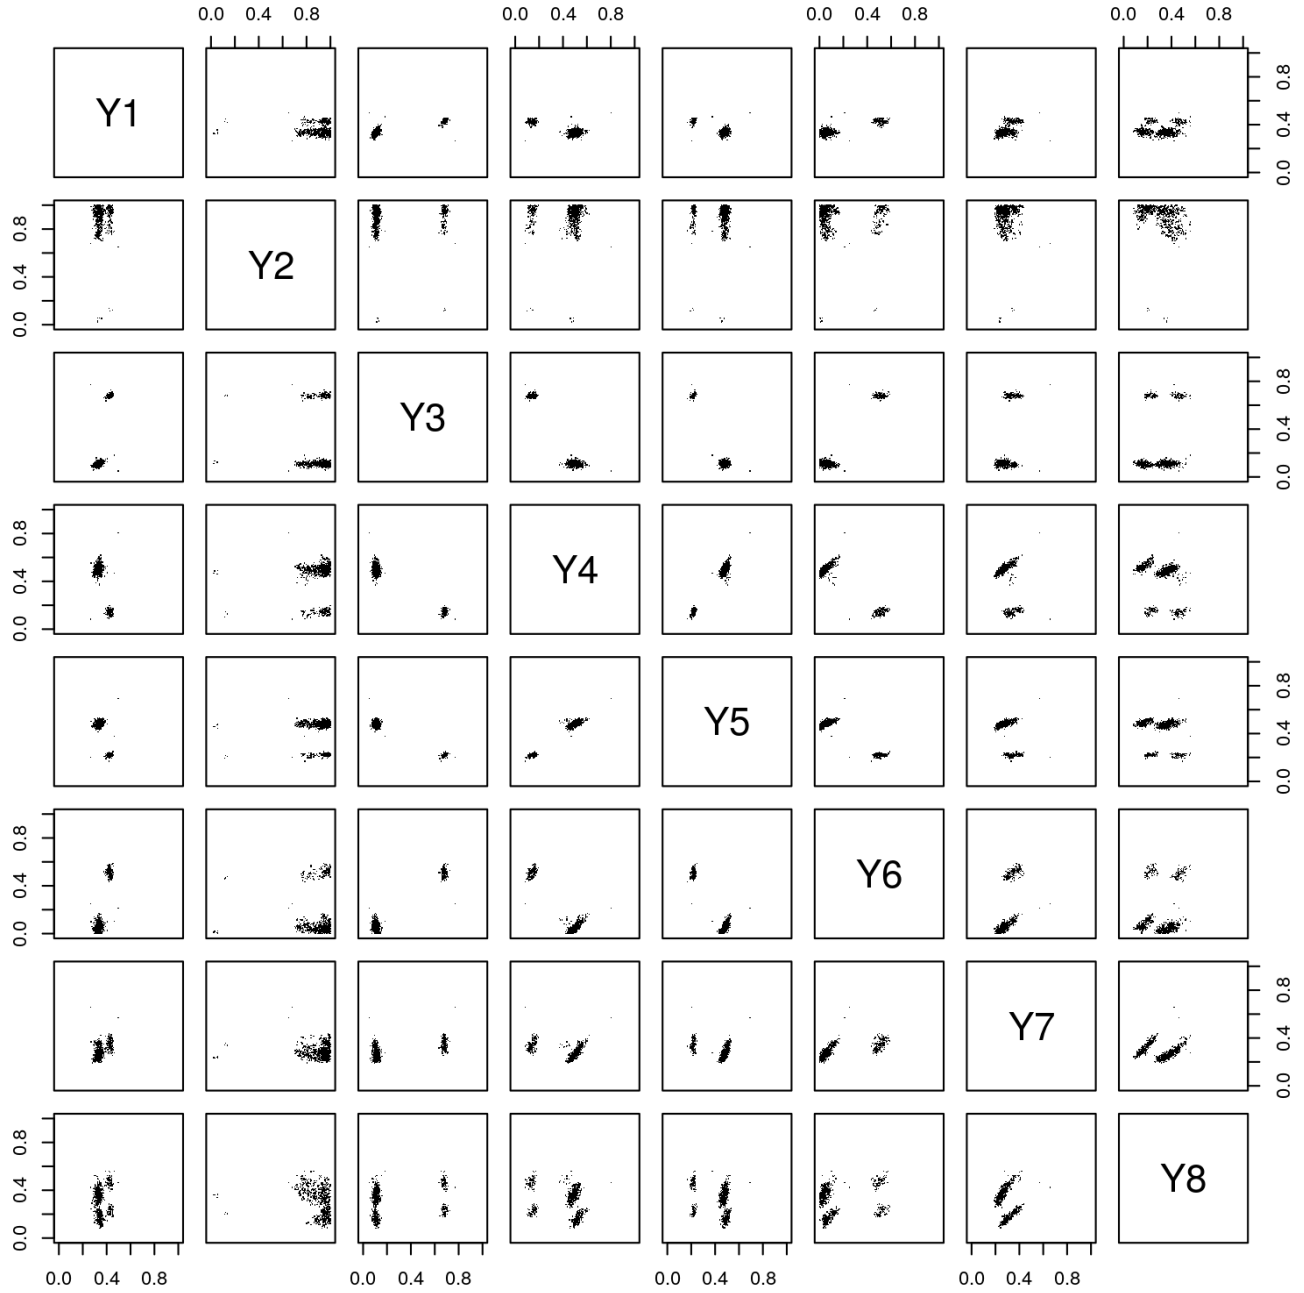

Figure S-8: The pairwise joint distributions of the posterior draws for the  $y$ -coordinates of the sensor from one of the twelve Markov chains shown in Figure S-7.

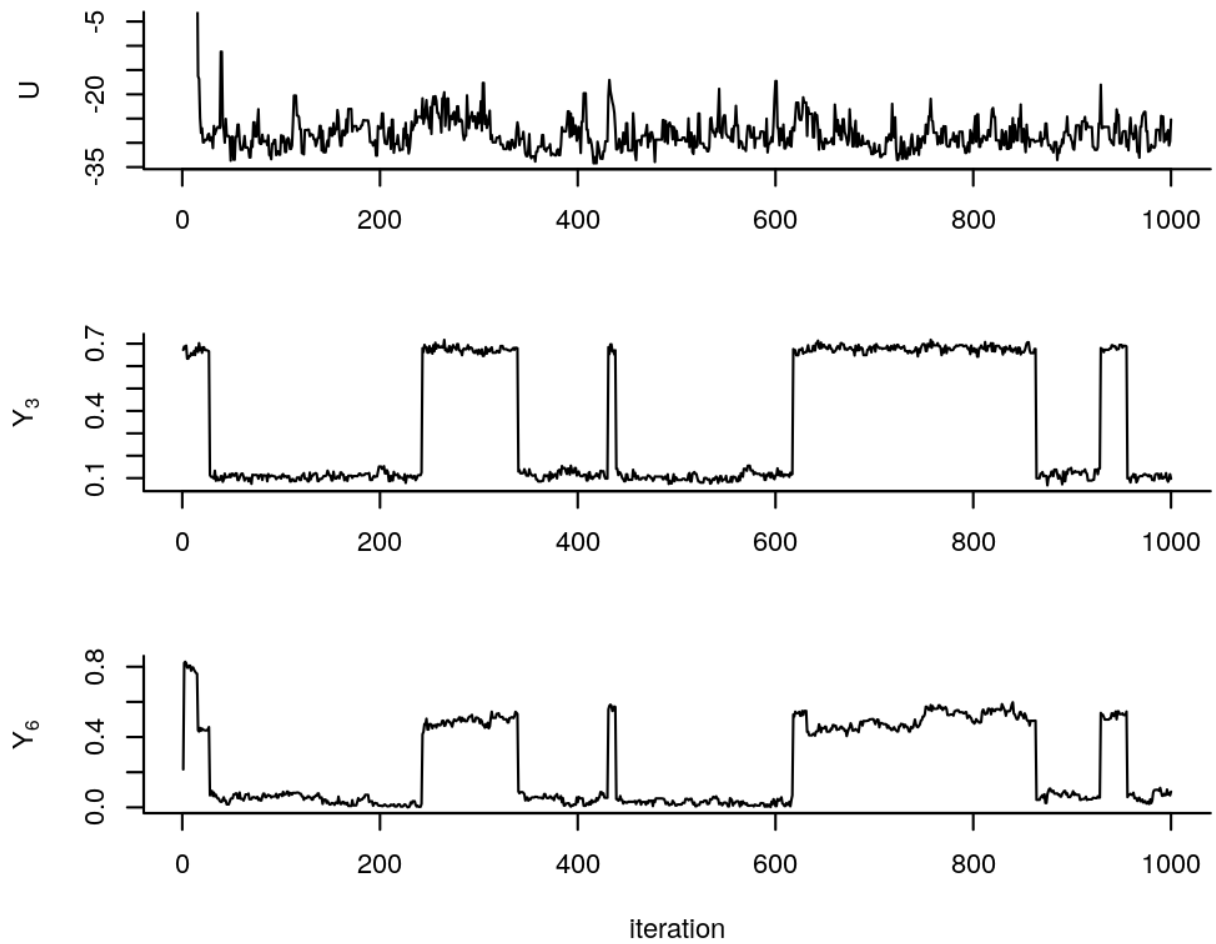

Figure S-9: The traceplot of the potential energy  $U$  and the  $y$ -coordinates of the third and the sixth sensors for the Markov chain shown in Figure S-8.

### S3.3 $\eta_k = \eta_* \{1 - \cos(2\pi k/K)\}$ with $\eta_* = 3$

Figures S-10–S-12 show that the Markov chains constructed by Algorithm 1 when the maximum mass scale factor is equal to  $e^{4\eta_*} = e^{12}$  can explore the two dominant modes of the posterior distribution.

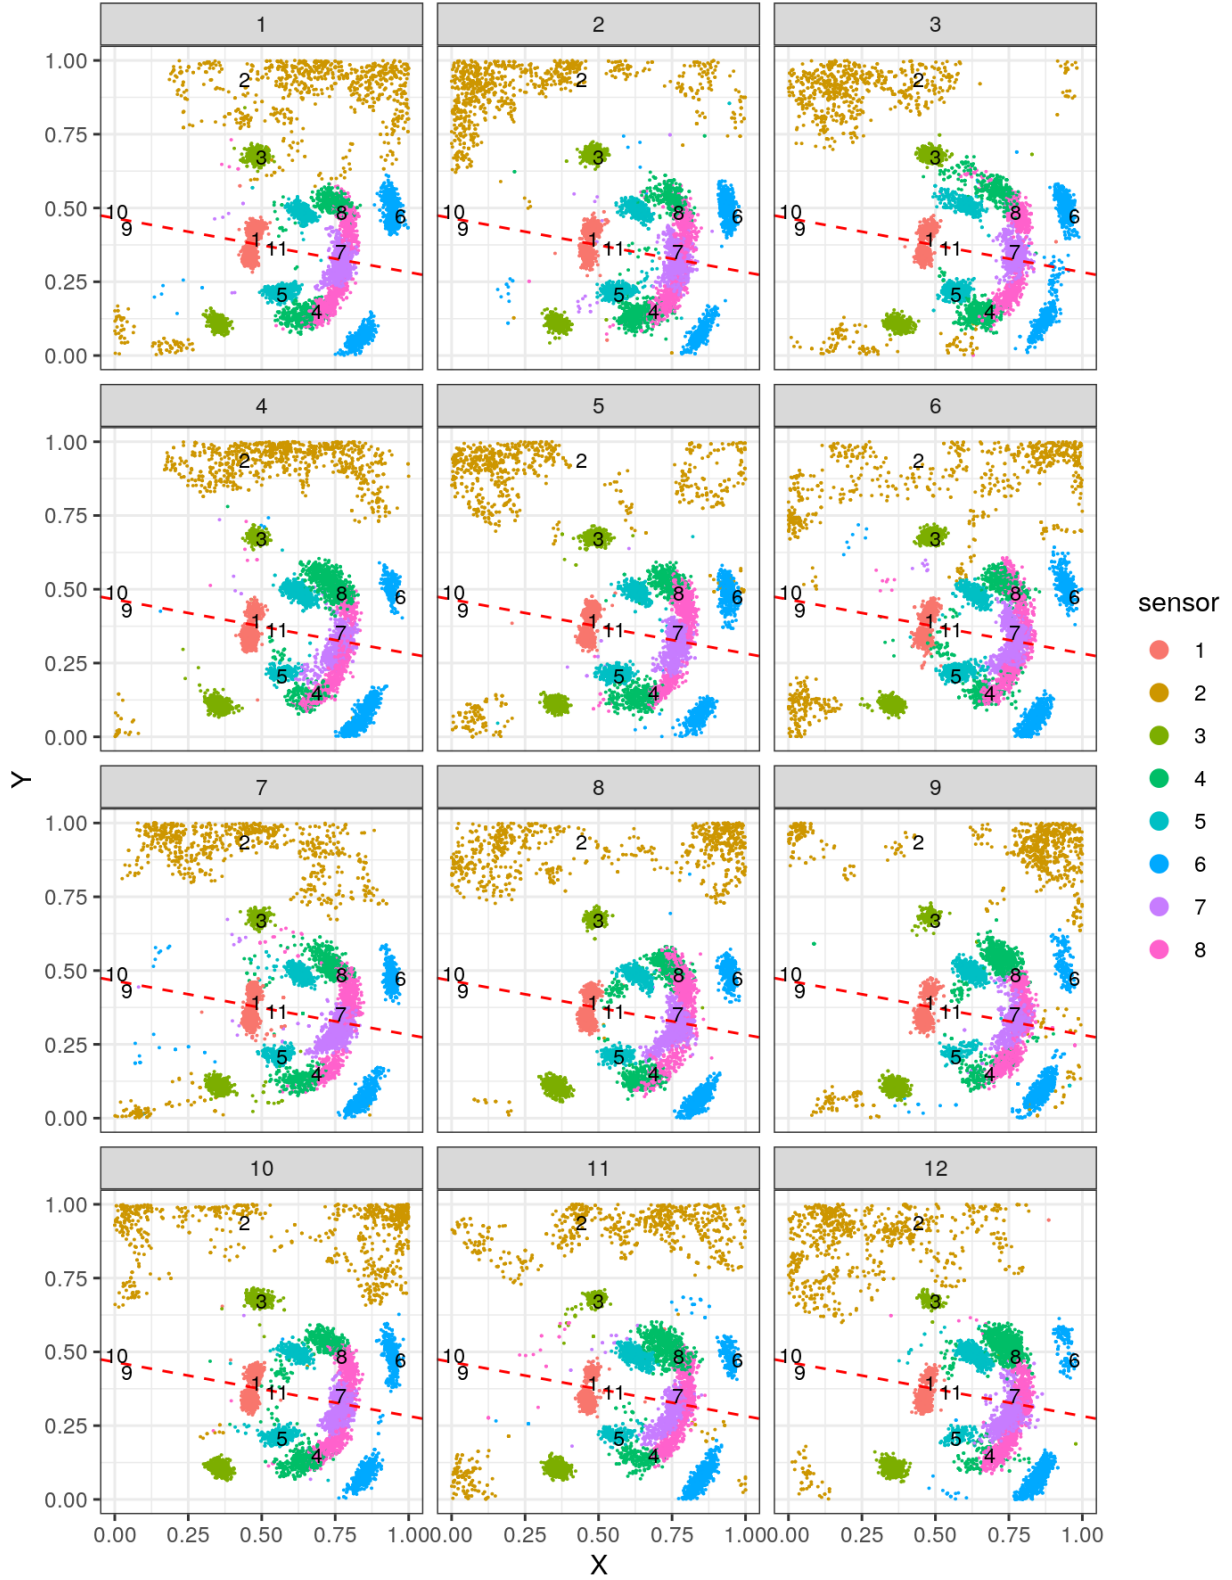

Figure S-10: The marginal posterior draws for the sensor locations from twelve independent Markov chains constructed using Algorithm 1 where  $\eta_k = \eta_* \{1 - \cos(2\pi k/K)\}$  with  $\eta_* = 3$  and  $K = 2000$ . The true location of each sensor is marked on the plot by its number. Sensors 9, 10, and 11 had known locations.

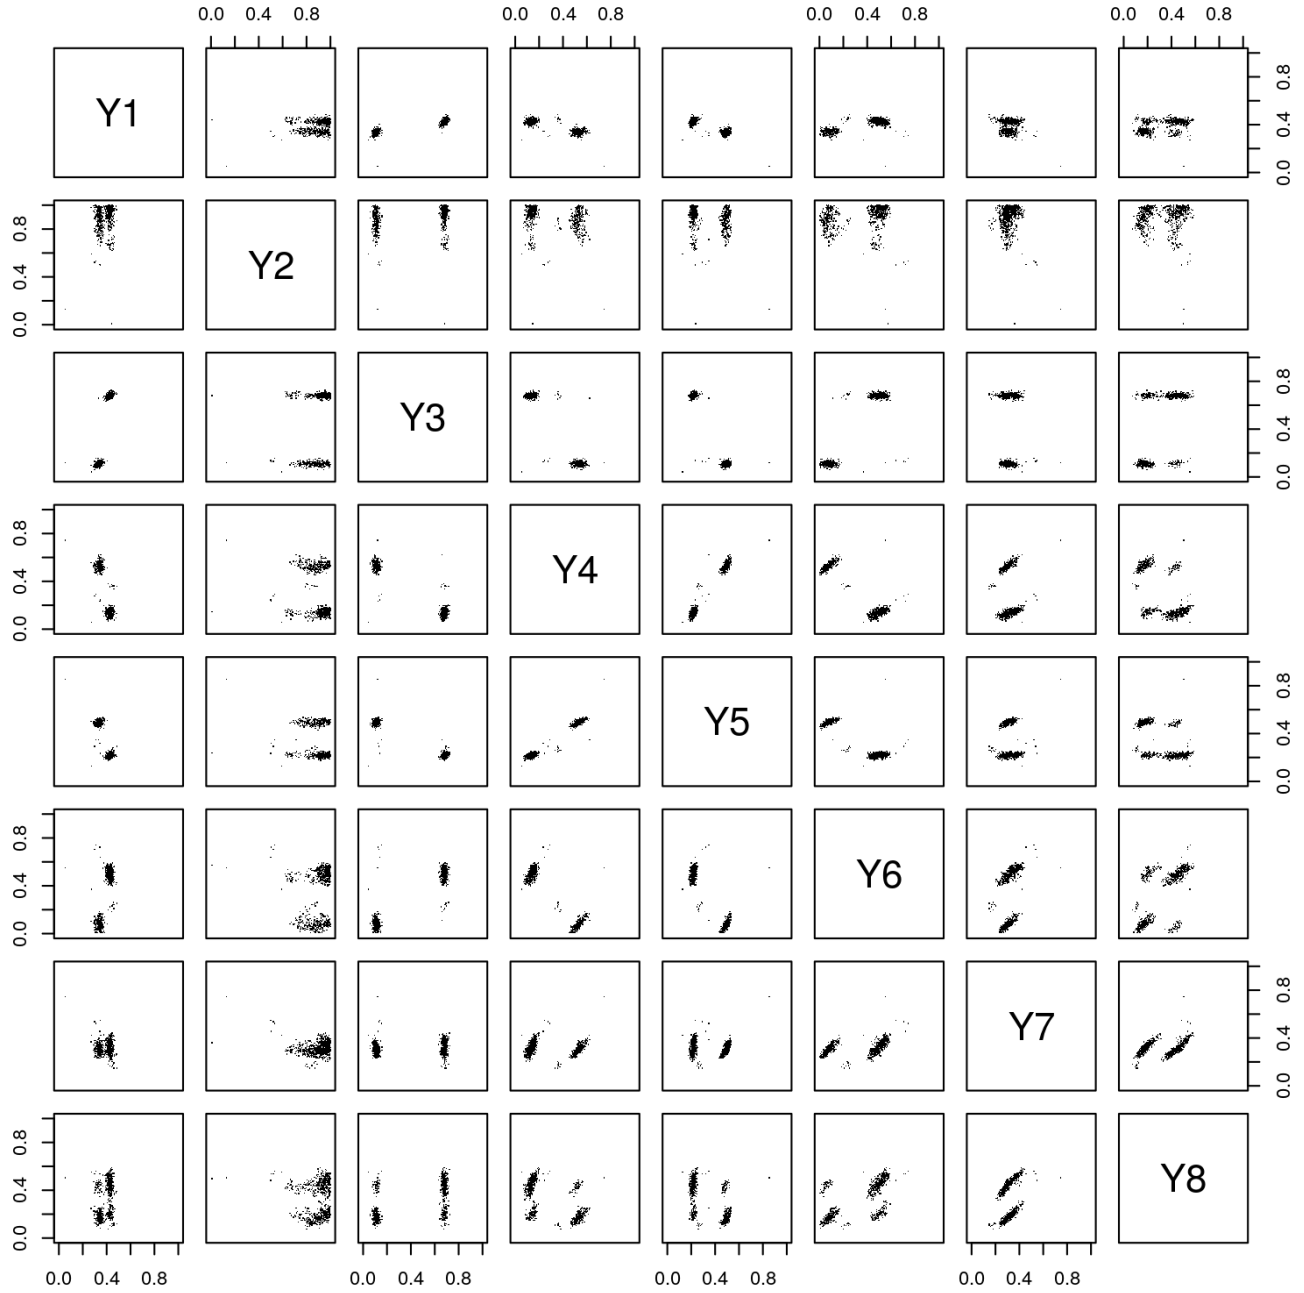

Figure S-11: The pairwise joint distributions of the posterior draws for the  $y$ -coordinates of the sensor from one of the twelve Markov chains shown in Figure S-10.



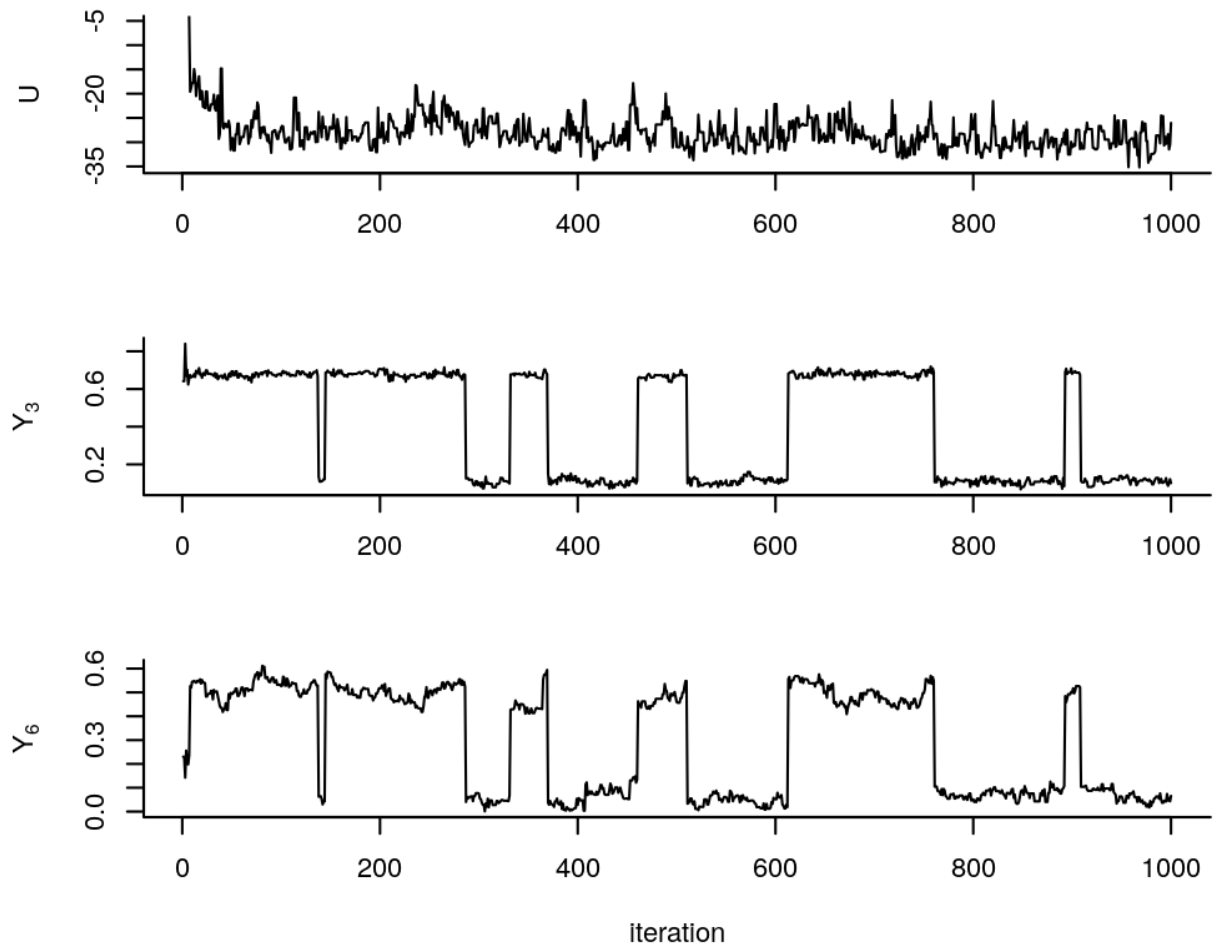

Figure S-12: The traceplot of the potential energy  $U$  and the  $y$ -coordinates of the third and the sixth sensors for the Markov chain shown in Figure S-11.

## Supplementary References

- Neal, R. M. (1996) Sampling from multimodal distributions using tempered transitions. *Statistics and computing*, **6**, 353–366.
- Park, J. and Atchadé, Y. (2020) Markov chain monte carlo algorithms with sequential proposals. *Statistics and Computing*, **30**, 1325–1345.
